# Supplementary material for: How Many Simultaneous Beamformers are Needed for Integrated Sensing and Communications?
Source: arXiv:2507.14982 source file (2026-06-16)
Supplement: Supplementary file 1 [file appendices.tex]

\section{Derivation of the BFIM expression}
\label{Appen:BFIM}
First, note that we may factor $f(\mathbf{X}, \mathbf{Y}_\text{s}, \boldsymbol{\eta})$ as follows
\begin{equation}\label{eq:pdf_factorization}
    f(\mathbf{X}, \mathbf{Y}_\text{s}, \boldsymbol{\eta}) = f(\boldsymbol{\eta}) \prod_{q = 1}^{\Upsilon} f(\mathbf{x}[q]) f\left(\mathbf{y}_\text{s}[q] \big{|} \mathbf{x}[q],  \boldsymbol{\eta}\right),
\end{equation}
where the above relation follows directly by noting that the random vectors $\boldsymbol{\eta}, \mathbf{x}[1], \ldots, \mathbf{x}[\Upsilon]$ are independent of each other, and that $\mathbf{y}_\text{s}[q]$ depends only on the current $\mathbf{x}[q]$ and $\boldsymbol{\eta}$. Using~\eqref{eq:pdf_factorization}, we can write the BFIM elements in~\eqref{eq:BFIM} as the following sum $[\mathbf{J}_{\mathbf{V}}]_{ij} = [\mathbf{C}]_{ij} + [\mathbf{T}_{\mathbf{V}}]_{ij}$, where $\mathbf{C}$ and $\mathbf{T}_{\mathbf{V}}$ are chosen as follows: %we choose $\mathbf{C}$ and $\mathbf{T}_\mathbf{V}$ such that
\begin{equation}~\label{eq:C_elements}
        [\mathbf{C}]_{ij} = - \mathbb{E}\left[ \frac{\partial^2 \log\left( f(\boldsymbol{\eta})\cdot  \prod_{q = 1}^{\Upsilon} f(\mathbf{x}[q]) \right) }{\partial \eta_i \partial \eta_j }\right]
\end{equation}
and
\begin{equation}~\label{eq:T_elements}
[\mathbf{T}_\mathbf{V}]_{ij} = -  \mathbb{E}\left[ \frac{\partial^2 \log \prod_{q = 1}^\Upsilon f(\mathbf{y}_\text{s}[q]\big{|} \mathbf{x}[q], \boldsymbol{\eta}) }{\partial \eta_i \partial \eta_j }\right]. %+ \mathbb{E}\left\{ \frac{\partial^2 \log f( \mathbf{x}[t] ) }{\partial \eta_i \partial \eta_j }\right\}
\end{equation}
Since $\mathbf{x}[q]$ is independent of $\boldsymbol{\eta}$, we can simplify~\eqref{eq:C_elements} as follows
\begin{subequations}
    \begin{align}
        [\mathbf{C}]_{ij} &= - \mathbb{E}\left[ \frac{\partial^2 \log f(\boldsymbol{\eta}) }{\partial \eta_i \partial \eta_j }\right] - \sum_{n = 1}^{\Upsilon} \mathbb{E}\left[ \frac{\partial^2 \log f( \mathbf{x}[q] ) }{\partial \eta_i \partial \eta_j }\right] \label{eq:C_linea}  \\
        &= - \mathbb{E}\left[ \frac{\partial^2 \log f(\boldsymbol{\eta}) }{\partial \eta_i \partial \eta_j }\right],
       \end{align} \end{subequations}
since the second term in~\eqref{eq:C_linea} is zero due to the independence of $\boldsymbol{\mathbf{x}[q]}$ and $\boldsymbol{\eta}$. This shows that $\mathbf{C}$ has the desired form. For $\mathbf{T}_{\mathbf{V}}$ in~\eqref{eq:T_elements}, it is easy to see that $f(\mathbf{y}_\text{s}[q]\big{|} \mathbf{x}[q], \boldsymbol{\eta})$ is a Gaussian distribution $\mathcal{CN}\left(\mathbf{G}^{(\boldsymbol{\eta})} \mathbf{x}[q], \sigma^2 \mathbf{I}_{N_\text{R}}\right)$. Using the law of total expectation, we can write
\begin{subequations}
\begin{align}
    [\mathbf{T}_{\mathbf{V}}]_{ij} &{=} \sum_{q = 1}^\Upsilon \mathbb{E}_{\mathbf{x}[q], \boldsymbol{\eta}} \Biggl[ \mathbb{E}\Biggl[  \frac{-\partial^2 \log f(\mathbf{y}_\text{s}[q]\big{|} \mathbf{x}[q], \boldsymbol{\eta}) }{\partial \eta_i \partial \eta_j } \Biggr| \mathbf{x}[q], \boldsymbol{\eta} \Biggr] \Biggr] \\ 
	&{=} \frac{2}{\sigma^2} \sum_{q = 1}^\Upsilon \mathbb{E}_{\mathbf{x}[q], \boldsymbol{\eta}} \Re\biggl\{\Tr\left( \dot{\mathbf{G}}_i^\textsf{H} \dot{\mathbf{G}}_j \mathbf{x}[q] \mathbf{x}^\textsf{H}[q]\right) \biggr\} \label{eq:T_V_line_b} \\
    &= \frac{\Upsilon}{\sigma^2} \Tr\left( \mathbb{E}_{\boldsymbol{\eta}} \left[ \dot{\mathbf{G}}_i^\textsf{H} \dot{\mathbf{G}}_j + \dot{\mathbf{G}}_j^\textsf{H} \dot{\mathbf{G}}_i\right] \mathbf{V}\mathbf{V}^\textsf{H}\right) \label{eq:T_V_line_c}
\end{align}
\end{subequations}
where~\eqref{eq:T_V_line_b} follows from the BFIM of Gaussian signals~\cite{kay1993fundamentals} and~\eqref{eq:T_V_line_c} uses the fact that $\mathbb{E}\left[\mathbf{x}[q] {\mathbf{x}[q]}^\textsf{H}\right] = \mathbf{V} \mathbf{V}^\textsf{H}$.

\section{Proof of Lemma~\ref{lem:quad_eq_sol_IC}}\label{appen:quad_eq_sol_IC} 

The first step is to express the BFIM and SINR constraints in~\eqref{eq:BFIM_SINR} as quadratic equations in $\left\{d_k\right\}$ and $\mathbf{U}_\text{s}$. For the BFIM constraint, we have the following $L(L + 1)/2$ quadratic equations in $\mathbf{V}'$ due to the symmetric nature of $\mathbf{J}$
\begin{equation}\label{eq:reform_BFIM}        \mathbf{J}_{\mathbf{V}'} = \mathbf{J} ~ \Leftrightarrow \Tr{\left(\mathbf{\tilde{G}}_{ij} \mathbf{V}' {\mathbf{V}'}^\mathsf{H}\right)} = t_{ij}, ~ 1 \leq i \leq j \leq L, 
        \end{equation}
        with $t_{ij} \triangleq \tfrac{\sigma^2}{\Upsilon}\left([\mathbf{J}]_{ij} - [\mathbf{C}]_{ij}\right)$. Further,  we have the following $K$ quadratic equations for the SINR constraints %amount to satisfying $K$ equations
\begin{equation}\label{eq:reform_SINR}        \text{vSINR}^\text{IC}_{\mathbf{V}'} = \boldsymbol{\gamma}' \Leftrightarrow \frac{|\mathbf{h}_k^\mathsf{H}\mathbf{v}'_k|^2}{\gamma_k'} - \sum_{n \neq k} |\mathbf{h}_k^\mathsf{H} \mathbf{v}'_{n} |^2  = \sigma^2, \quad \forall k.
        \end{equation}
Plugging the rank reduction structure \eqref{eq:transformation_IC}-\eqref{eq:transformation_IC2} into \eqref{eq:reform_BFIM}-\eqref{eq:reform_SINR}, we obtain the following set of quadratic equations 
in $\left\{d_k\right\}$ and $ \mathbf{U}_\text{s}$
\begin{align}
            \sum_k |d_k|^2 {\mathbf{\hat{v}}_k}^\mathsf{H} \tilde{\mathbf{G}}_{ij}\mathbf{\hat{v}}_k {+} \Tr\Big(  \tilde{\mathbf{G}}_{ij}\mathbf{\hat{V}}_\text{s} \mathbf{U}_\text{s} \mathbf{U}_\text{s}^\mathsf{H}{\mathbf{\hat{V}}_\text{s}}^\mathsf{H} \Big) & = t_{ij}, \forall i, j \label{eq:BFIM2} \\
            \frac{ |d_k\mathbf{h}_k^\mathsf{H} \mathbf{\hat{v}}_k|^2}{\gamma_k'}  {-} \sum_{n \neq k} |d_n\mathbf{h}_k^\mathsf{H} \mathbf{\hat{v}}_n|^2 
             & = \sigma^2,~ \forall k. \label{eq:SINR2} 
\end{align}
%Whenever , it is always possible to construct $\mathbf{V}'$ with fewer sensing beamformers and to attain the same BFIM and SINRs. We now show that this is possible whenever.
%In order to maintain the values of BFIM and SINR, we need to find $\{d_k\}$
In addition to~\eqref{eq:BFIM2}-\eqref{eq:SINR2}, we also require $\mathbf{U}_\text{s}$ to be a tall matrix to ensure that $\mathbf{V}'$ has fewer sensing beamformers. 

Next, we aim to prove the existence of $\{d_k\}$ and tall matrix $\mathbf{U}_\text{s}$ that solve~\eqref{eq:BFIM2}-\eqref{eq:SINR2}, provided that condition~\eqref{eq:IC_condition} holds. Subsequently, we prove that the $\mathbf{V'}$ obtained by such $\{d_k\}$ and $\mathbf{U}_\text{s}$ also satisfies the power constraint.

%We show that~\eqref{eq:BFIM2}-\eqref{eq:SINR2} must have a solution as long as $\hat{N}_\text{s}$ satisfies~\eqref{eq:IC_condition}. %Subsequently, we prove that such $\mathbf{V'}$ also satisfies the power constraint.
Define $a_k = 1 - |d_k|^2$ and $\mathbf{M}_\text{s} = \mathbf{I}_{N_\text{s}} - \mathbf{U}_\text{s} \mathbf{U}_\text{s}^\mathsf{H}$. Since $\mathbf{\hat{V}}$ also achieves $\left(\mathbf{J}, \boldsymbol{\gamma}'\right)$, % ~\eqref{eq:reform_BFIM}-\eqref{eq:reform_SINR}, 
        we can express \eqref{eq:BFIM2}-\eqref{eq:SINR2} in terms of the new variables $\{a_k\}$ and $\mathbf{M}_\text{s}$ as follows:
        %Substituting the new variables into~\eqref{eq:BFIM2}-\eqref{eq:SINR2} and using the fact that $\hat{\mathbf{V}}$ also satifies~\eqref{eq:BFIM_const}-\eqref{eq:SINR_const}, we get the equivalent system of linear equations
%\begin{subequations}\label{eq:lin_system}
\begin{align}
\sum_k a_k {\mathbf{\hat{v}}_k}^\mathsf{H} \tilde{\mathbf{G}}_{ij}\mathbf{\hat{v}}_k + \Tr\Big(  \tilde{\mathbf{G}}_{ij}\mathbf{\hat{V}}_\text{s} \mathbf{M}_\text{s} {\mathbf{\hat{V}}_\text{s}}^\mathsf{H} \Big) & = 0, \forall i, j \label{eq:linear_BFIM} \\
\frac{a_k|\mathbf{h}_k^\mathsf{H} \mathbf{\hat{v}}_k|^2}{\gamma_k'} - \sum_{n \neq k}a_n |\mathbf{h}_k^\mathsf{H} \mathbf{\hat{v}}_n|^2 
             & = 0, ~\forall k. \label{eq:linear_SINR}
\end{align}
%\end{subequations}
This is a linear system of equations.  In addition, we have the following conditions due to the definitions of $\{a_k\}$ and $\mathbf{M}$:
\begin{equation}\label{eq:extra_constraints}
            \mathbf{I}_{N_\text{s}} - \mathbf{M}_\text{s} \succcurlyeq 0, ~~{\mathbf{I}_{N_\text{s}} - \mathbf{M}_\text{s} ~ \text{singular}}, ~~ 1 - a_k \geq 0, ~~ \forall k. 
        \end{equation}
%The first and last conditions are needed to ensure that we can retrieve $\mathbf{U}_\text{s}$ and $d_1, \ldots, d_K$. 
Note that $\mathbf{I}_{N_\text{s}} - \mathbf{M}_\text{s} = \mathbf{U}_\text{s} \mathbf{U}_\text{s}^\mathsf{H}$ must be singular since $\mathbf{U}_\text{s}$ is restricted to be a tall matrix.
        
The set of equations \eqref{eq:linear_BFIM}-\eqref{eq:linear_SINR} comprise a linear homogeneous system with $K + L(L+1)/2$ equations and $K + N_\text{s}^2$ real unknowns. There are $K$ equations from the SINR constraints and $L(L+1)/2$ equations from the BFIM constraint (due to symmetry), and there are $K$ real variables $a_1, \ldots, a_K$ and $N_\text{s}^2$ real variables from the Hermitian matrix $\mathbf{M}_\text{s}$. 
So if~\eqref{eq:IC_condition} holds, the number of unknowns exceeds the number of equations and such system must have a solution $a'_1, \ldots, a'_K, \mathbf{M}'_\text{s}$, which are not all zero. This solution can be scaled as follows
\begin{equation}~\label{eq:scaling}
\mathbf{M}_\text{s} = \frac{1}{\delta} \mathbf{M}_\text{s}', \quad a_k = \frac{a_k'}{\delta}, \quad \forall k,
\end{equation}
to additionally satisfy \eqref{eq:extra_constraints}. Here, $\delta$ is chosen to satisfy 
\begin{equation}\label{eq:delta}
|\delta| = \max\{|a_1'|, \ldots, |a_K'|, |\delta_1'|, \ldots, |\delta_{\hat{m}}'|\},
\end{equation}
so either $\delta = a_k'$ for some $k$ or $\delta=\delta_m'$ for some $m$,
where $\delta_1', \ldots, \delta_{\hat{N}_\text{s}}'$ are the eigenvalues of $\mathbf{M}'_\text{s}$. 
Note that $\delta \neq 0$ since $\{a'_k\}$ and $\{\delta_m'\}$ are not all zero.

It is straightforward to verify that $\{a_k\}$ and $\mathbf{M}_\text{s}$ defined in~\eqref{eq:scaling} must satisfy $\mathbf{I}_{N_\text{s}}- \mathbf{M}_\text{s} \succcurlyeq 0$ and $1 - a_k \geq 0, \forall k$. The fact that $\mathbf{I}_{N_\text{s}} - \mathbf{M}_\text{s}$ is singular is established by contradiction. Suppose that $\mathbf{I}_{N_\text{s}} - \mathbf{M}_\text{s}$ is nonsingular, then by~\eqref{eq:scaling}, we must have $1 - \tfrac{\delta_m}{\delta} > 0$ for all $m =\{1, \ldots, N_\text{s}\}$, which implies that $\delta = a_i$ for some $i$. In this case, the corresponding $d_i$ is zero and $\mathbf{v}_i'$ in~\eqref{eq:transformation_IC} is the all-zero vector. However, this cannot happen since it violates the SINR constraint, because $\gamma_k > 0, \forall k$ by assumption.

Given a solution of~\eqref{eq:linear_BFIM}-\eqref{eq:extra_constraints}, we can recover $\{d_k\}$ and $\mathbf{U}_\text{s}$ and subsequently find $\mathbf{V}'$ that attains $\left(\mathbf{J}, \boldsymbol{\gamma}'\right)$. We claim that such $\mathbf{V}'$ automatically %solving~\eqref{eq:lin_system}-\eqref{eq:extra_constraints} 
has the same power as $\mathbf{\hat{V}}$. 
To see why, recall that $\mathbf{\hat{V}}$ is a solution to the problem
$\mathcal{P}_{N}^\text{IC}$, which has strong duality by assumption. The dual problem of  $\mathcal{P}_{N}^\text{IC}$ is the following
\begin{subequations}\label{prob:dual_IC}
\begin{align}
    \underset{\{\nu_{i, j}\}, \{\mu_k\}}{\mathrm{maximize}} ~~ &\sum_{i \le j} \nu_{i,j} t_{i, j} + \sigma^2 \sum_{k} \mu_k \\
    \mathrm{subject \; to} ~~& \mathbf{I}_N \succcurlyeq \sum_{i \le j} \nu_{i, j} \tilde{\mathbf{G}}_{i, j} \\
    &\mathbf{I}_N \succcurlyeq \sum_{i \le j} \nu_{i, j} \tilde{\mathbf{G}}_{i, j}  {+} \frac{\mu_k}{\gamma_k} \mathbf{h}_k \mathbf{h}_k^\mathsf{H}  {-} \sum_{n \neq k} {\mu_n} \mathbf{h}_n \mathbf{h}_n^\mathsf{H} \\
    & \mu_k \geq 0, \quad \forall k,
\end{align}
\end{subequations}
%First, because $(\mathbf{J}, \boldsymbol{\gamma}) \in \mathcal{A}_{N_\text{T}}^\text{IC}$, we must have $\Tr(\mathbf{\hat V}\mathbf{\hat V}^\mathsf{H}) \leq P$.
%The latter statement can be proved by showing that its SDR is tight using the technique in \cite{Liu2020joint}. 
%    It can be shown that has strong duality (this can be proved by showing that its SDR is tight), so that the following first-order conditions hold for $\hat{\mathbf{V}} \triangleq [ \hat{\mathbf{v}}_1, \ldots, \hat{\mathbf{v}}_K, \hat{\mathbf{V}_\text{s}}]$.
%\begin{lemma}\label{lem:reduction}
where $\{\nu^*_{i, j}\}_{1 \leq i \le j \leq L}$ and $\{\mu^*_k\}_{1\leq k \leq K}$ are the dual variables associated with the BFIM  and SINR constraints, respectively. By strong duality, it follows that there exist optimal dual variables $\{\nu^*_{i, j}\}_{1 \leq i \le j \leq L}$ and $\{\mu^*_k\}_{1\leq k \leq K}$ such that the optimality conditions as written below are satisfied:
           % \begin{subequations}
\begin{align}
\mathbf{\hat{V}}_\text{s} &= \left(\sum_{i \le j} \nu^*_{i, j} \tilde{\mathbf{G}}_{i, j} \right)  \mathbf{\hat{V}}_\text{s} \label{eq:CS_vs} \\
\mathbf{\hat{v}}_k & = \left(\sum_{i \le j} \nu^*_{i, j} \tilde{\mathbf{G}}_{i, j}  + \frac{\mu^*_k}{\gamma_k} \mathbf{h}_k \mathbf{h}_k^\mathsf{H}  - \sum_{n \neq k} \mu^*_n \mathbf{h}_n \mathbf{h}_n^\mathsf{H}\right) \mathbf{\hat{v}}_k, \forall k \label{eq:CS_vk}
%\mu_k^* \sigma^2 &= \mu_k^* \left(\frac{|\mathbf{h}_k^\mathsf{H}\mathbf{\hat{v}}_k|^2}{\gamma_k} - \sum_{n \neq k} |\mathbf{h}_k^\mathsf{H} \mathbf{\hat{v}}_{n} |^2 \right) , \quad \forall k
\end{align}
and that the primal optimum is equal to the dual optimum
\begin{equation}
\sum_{i \le j} \nu^*_{i,j} t_{i, j} + \sigma^2 \sum_{k} \mu^*_k = \Tr\big(\mathbf{ \hat V} \mathbf{\hat V}^\mathsf{H}\big).
\end{equation} %\hfill $\blacksquare$
%            \begin{IEEEproof}
%                %Strong duality can be proved by showing that  $\mathcal{P}_{\mathbf{J}, \boldsymbol{\gamma}}$ has a tight SDR. 
%                We omit the details for space limitations. 
%        \end{IEEEproof}
%        \end{lemma}
%        To prove this claim, we use Lemma~\ref{lem:reduction}. If we
Multiplying both sides of \eqref{eq:CS_vk} from the left by $|d_k|^2 \mathbf{\hat{v}}_k^\mathsf{H}$ and both sides of \eqref{eq:CS_vs} from the left by $\mathbf{\hat{V}}^\mathsf{H}_\text{s}\mathbf{U}^\mathsf{H}\mathbf{U}$, and summing the $K$ equations in \eqref{eq:CS_vk} together with \eqref{eq:CS_vs}, we get
\begin{align}
\Tr\left({\mathbf{V}'}^\mathsf{H} {\mathbf{V}'}\right) & = \sum_{i \le j} \nu^*_{i, j} \Tr\left( {\mathbf{V}'}^\mathsf{H}\tilde{\mathbf{G}}_{i,j} {\mathbf{V}'}  \right) 
\nonumber\\
        & \qquad +  
 \sum_k \mu^*_k \left( \frac{|\mathbf{h}_k^\mathsf{H} \mathbf{v}'_k|^2}{\gamma_k}  - \sum_{n \neq k} |\mathbf{h}_k^\mathsf{H} \mathbf{v}'_n|^2 \right) \nonumber \\
 & = \sum_{i \le j} \nu^*_{i, j} t_{i, j}  \nonumber \\
 & \qquad +  
 \sum_k \mu^*_k \left( \frac{|\mathbf{h}_k^\mathsf{H} \mathbf{v}'_k|^2}{\gamma_k'}  - \sum_{n \neq k} |\mathbf{h}_k^\mathsf{H} \mathbf{v}'_n|^2 \right) \nonumber \\
            & = \sum_{i \le j} \nu^*_{i, j} t_{i, j} +  \sigma^2 \sum_k \mu^*_k \nonumber \\
        &=\Tr\left({\mathbf{\hat{V}}}^\mathsf{H} {\mathbf{\hat{V}}}\right),
\end{align}
where we make use of \eqref{eq:reform_BFIM} and \eqref{eq:reform_SINR}. Note that in the second equality we replace $\gamma_k$ with $\gamma_k'$ since $\mu_k^*$ must be zero whenever $\gamma_k' \neq \gamma_k$ due to complementary slackness. %, and %also the fact that because $(\mathbf{J}, \boldsymbol{\gamma}) \in \mathcal{A}^{(N_\text{T})}$, we must have $\Tr(\mathbf{\hat V}\mathbf{\hat V}^\mathsf{H}) \leq P$.
%In other words, $\mathbf{V}'$ additionally satisfies the power constraint. 
%Thus, $\mathbf{V}'$ has power at most $P$. 
To summarize, provided that the number of sensing beamformers satisfies \eqref{eq:IC_condition}, it is always possible to reduce the number of sensing beamformers while satisfying \eqref{eq:BFIM_SINR}.
        
Finally, we prove that i) $\mathbf{V}'$ is an optimal
solution of $\mathcal{P}_{N'}^\text{IC}$; and ii) $\mathcal{P}_{N'}^\text{IC}$ must also have strong duality. The former holds because the optimal value of $\mathcal{P}_{N'}^\text{IC}$
must be less than or equal to that of $\mathcal{P}_{N}^\text{IC}$ (since $N'
 < N$), but 
$\mathbf{V'}$ achieves the the same power as $\mathbf{\hat{V}}$, which is the optimal value of $\mathcal{P}_{N}^\text{IC}$.
So it must be an optimal solution of $\mathcal{P}_{N'}^\text{IC}$. The latter holds because $\mathcal{P}_{N'}^\text{IC}$ and $\mathcal{P}_{N}^\text{IC}$ give rise to 
the same dual problem~\eqref{prob:dual_IC} and both attain the same minimum. %The SDR of this type of 
%nonconvex optimization problem gives the optimal value of its dual problem.
Since $\mathcal{P}_{N}^\text{IC}$ has strong duality, $\mathcal{P}_{N'}^\text{IC}$ must also have strong duality.

\section{Proof of Strong Duality for $\mathcal{P}^\text{IC}_{N_\text{T} + K}$ and $\mathcal{P}^\text{NIC}_{N_\text{T} + K}$}\label{Appen:strong_duality}
The proof follows from a standard trick used to establish strong duality for ISAC problems with a similar structure; see~\cite{LiuFCRB2022, HuaOptimal2023}, and \cite[Theorem 1]{Liu2020joint}. We include the proof here to keep this paper self-contained. %To keep this paper self-contained, we use the same trick here to show that  $\mathcal{P}^\text{IC}_{N_\text{T} + K}$ also has strong duality. 
First consider  $\mathcal{P}^\text{IC}_{N_\text{T} + K}$. The SDR obtained by defining $\mathbf{R} = \mathbf{V} \mathbf{V}^\mathsf{H}$, $\mathbf{R}_k = \mathbf{v}_k \mathbf{v}_k^\mathsf{H}$, and dropping the rank-one constraints on $\mathbf{R}_k$ is
\begin{subequations} \label{prob:P_SDR}
         \begin{align}
\underset{\mathbf{R}, \mathbf{R}_1, \ldots, \mathbf{R}_K}{\mathrm{minimize}}~~~&\Tr{\left(\mathbf{R}\right)} \\
            {\mathrm{subject\; to}}~~&\mathbf{J}_{\mathbf{R}} = \mathbf{J}, \\
            &\frac{1}{\gamma_k} \mathbf{h}_k^\mathsf{H}\mathbf{R}_k \mathbf{h}_k - \sum_{n \neq k } \mathbf{h}_k^\mathsf{H}\mathbf{R}_n \mathbf{h}_k \geq \sigma^2, \forall k \label{eq:kth_sINR}\\
            & \mathbf{R} \succcurlyeq \sum_k \mathbf{R}_k, \quad   \mathbf{R}_k \succcurlyeq 0, \quad \forall k,
         \end{align}
        \end{subequations}
where  $\mathbf{J}_\mathbf{R}$ denotes, with a slight abuse of notation, the BFIM matrix expressed in $\mathbf{R}$ (i.e., with $\mathbf{V}\mathbf{V}^\textsf{H}$ replaced with $\mathbf{R}$ in~\eqref{eq:TV_elements}). 
The proof of strong duality follows from showing that the above relaxation is tight. That is, there exists an SDR solution $\mathbf{\tilde R}, \mathbf{\tilde{R}}_1, \ldots, \mathbf{\tilde{R}}_K$, with $\rank (\mathbf{\tilde{R}}_k) = 1$ for all $k$.  Let $\mathbf{\hat{R}}, \mathbf{\hat{R}}_1, \ldots, \mathbf{\hat{R}}_K$ be an arbitrary high-rank solution of the SDR. We construct $\mathbf{\tilde R}, \mathbf{\tilde{R}}_1, \ldots, \mathbf{\tilde{R}}_K$ as follows:
\begin{equation}\label{eq:rank_one_solution}
    \mathbf{\tilde R} = \mathbf{\hat R}, \quad \mathbf{\tilde{R}}_k = \frac{\mathbf{\hat{R}}_k \mathbf{h}_k \mathbf{h}_k^\mathsf{H} \mathbf{\hat{R}}_k}{\mathbf{h}_k^\mathsf{H} \mathbf{\hat{R}}_k \mathbf{h}_k }, \quad \forall k. 
\end{equation}
Clearly, $\mathbf{\tilde{R}}_1, \ldots, \mathbf{\tilde{R}}_K$ as given by~\eqref{eq:rank_one_solution} are all rank-one PSD matrices. The new solution attains the same power and BFIM as $\mathbf{\hat{R}}, \mathbf{\hat{R}}_1, \ldots, \mathbf{\hat{R}}_K$ since the overall covariance is the same. Further, we note that the following holds:
\begin{align}\label{eq:rank_one_conditions2}
\mathbf{h}_k^\mathsf{H}\mathbf{\hat{R}}_k \mathbf{h}_k  = \mathbf{h}_k^\mathsf{H}\mathbf{\tilde{R}}_k \mathbf{h}_k, \quad    \mathbf{\hat{R}}_k \succcurlyeq \mathbf{\tilde{R}}_k, \quad \forall k.
\end{align}
This is proved as follows. First, the equality is immediate from~\eqref{eq:rank_one_solution}. Let $\mathbf{w} \in \mathbb{C}^{N_\text{T}}$ be an arbitrary vector. Then,
\begin{equation}
    \mathbf{w}^\mathsf{H} \left( \mathbf{\hat{R}}_k - \mathbf{\tilde{R}}_k\right) \mathbf{w} = \mathbf{w}^\mathsf{H} \mathbf{\hat{R}}_k \mathbf{w} - \frac{\left| \mathbf{h}_k^\mathsf{H} \mathbf{\hat{R}}_k \mathbf{w} \right|^2}{\mathbf{h}_k^\mathsf{H} \mathbf{\hat{R}}_k \mathbf{h}_k } \geq 0.
\end{equation}
where the last inequality follows from the Cauchy-Schwarz inequality. This shows that $\mathbf{w}^\mathsf{H} \mathbf{\hat{R}}_k\mathbf{w} \geq \mathbf{w}^\mathsf{H}   \mathbf{\tilde{R}}_k\mathbf{w}$, for all $\mathbf{w}$. Or, equivalently, $\mathbf{\hat R}_k \succcurlyeq \mathbf{\tilde{R}}_k$.

Notice that~\eqref{eq:rank_one_conditions2} implies that, for the $k$-th SINR constraint in~\eqref{eq:kth_sINR}, the useful power term  remains the same when $\mathbf{\hat R}_k$ is replaced with $\mathbf{\tilde R}_k$. But the interference terms are reduced. Hence, the SINR constraints are also satisfied for the new solution. In particular,
\begin{align}
\frac{1}{\gamma_k} \mathbf{h}_k^\mathsf{H}\mathbf{\tilde R}_k \mathbf{h}_k - \sum_{n \neq k } \mathbf{h}_k^\mathsf{H}\mathbf{\tilde R}_n \mathbf{h}_k &= \frac{1}{\gamma_k} \mathbf{h}_k^\mathsf{H}\mathbf{\hat R}_k \mathbf{h}_k - \sum_{n \neq k } \mathbf{h}_k^\mathsf{H}\mathbf{\tilde R}_n \mathbf{h}_k \nonumber \\
&\geq \frac{1}{\gamma_k} \mathbf{h}_k^\mathsf{H}\mathbf{\hat R}_k \mathbf{h}_k - \sum_{n \neq k } \mathbf{h}_k^\mathsf{H}\mathbf{\hat R}_n \mathbf{h}_k \nonumber \\
&\geq \sigma^2.
\end{align}
Thus, $\mathbf{\tilde{R}}, \mathbf{\tilde{R}}_1, \ldots, \mathbf{\tilde{R}}_K$ is an optimal solution, and the SDR is tight.  Now, the SDR problem~\eqref{prob:P_SDR} enjoys strong duality since it is convex and satisfies Slater's condition. The latter statement can be proved by showing that its dual is strictly feasible. The proof of strong duality for $\mathcal{P}_{N_\text{T} + K}^\text{IC}$ readily follows by noting that problem~\eqref{prob:P_SDR} and $\mathcal{P}_{N_\text{T} + K}^\text{IC}$ give rise to the same dual.

The same proof above can be appropriately modified to show that $\mathcal{P}_{N_\text{T} +K}^\text{NIC}$ defined for the no interference cancellation scenarios, has strong duality. The SDR of  $\mathcal{P}_{N_\text{T} +K}^\text{NIC}$ is:
\begin{subequations} 
         \begin{align}
\underset{\mathbf{R}, \mathbf{R}_1, \ldots, \mathbf{R}_K}{\mathrm{minimize}}~~~&\Tr{\left(\mathbf{R}\right)} \\
            {\mathrm{subject\; to}}~~&\mathbf{J}_{\mathbf{R}} = \mathbf{J}, \\
            &\left( 1+ \frac{1}{\gamma_k}\right)\mathbf{h}_k^\mathsf{H}\mathbf{R}_k \mathbf{h}_k -\mathbf{h}_k^\mathsf{H}\mathbf{R} \mathbf{h}_k \geq \sigma^2, \forall k \\
            & \mathbf{R} \succcurlyeq \sum_k \mathbf{R}_k, \quad   \mathbf{R}_k \succcurlyeq 0, \quad \forall k,
\end{align}
\end{subequations}
For an arbitrary high-rank solution $\mathbf{\hat{R}}, \mathbf{\hat{R}}_1, \ldots, \mathbf{\hat{R}}_K$, the matrices defined in~\eqref{eq:rank_one_solution} constitute a solution with $\rank(\mathbf{\tilde{R}_k}) = 1$. Indeed, the power and BFIM remain the same since the covariance is the same. For the SINR constraints, we have
\begin{align}
\left(1 + \frac{1}{\gamma_k} \right) \mathbf{h}_k^\mathsf{H}\mathbf{\tilde R}_k \mathbf{h}_k &-\mathbf{h}_k^\mathsf{H}\mathbf{\tilde R} \mathbf{h}_k  \nonumber \\
&= \left(1 + \frac{1}{\gamma_k} \right) \mathbf{h}_k^\mathsf{H}\mathbf{\hat R}_k \mathbf{h}_k - \mathbf{h}_k^\mathsf{H}\mathbf{\hat R} \mathbf{h}_k \nonumber \\
&= \sigma^2.
\end{align}
The rest of the proof is similar to that of $\mathcal{P}_{N_\text{T} +K}^\text{IC}$.

\section{Proof of Lemma~\ref{lem:Ortho_Vs_NIC}}
\label{appen:Ortho_Vs_NIC}
      Our proof of the lemma is constructive. Since $(\mathbf{J}, \boldsymbol{\gamma}) \in \mathcal{A}_{N}^\text{NIC}$, problem $\mathcal{P}_N^\text{NIC}$ must have at least one solution.
        Let $\mathbf{\hat{V}} = [\mathbf{\hat{v}}_1, \ldots,  \mathbf{\hat{v}}_K, \mathbf{\hat{V}}_\text{s}] \in \mathbb{C}^{N_\text{T} \times N}$ denote an arbitrary solution of $\mathcal{P}_N^\text{NIC}$. To prove the lemma, we aim to construct another solution of $\mathcal{P}_N^\text{NIC}$ whose sensing beamformers are orthogonal to $\mathbf{h}_1, \ldots, \mathbf{h}_K$. Let us denote such a solution by $\mathbf{V}'= = \left[ \mathbf{v'}_1, \ldots, \mathbf{v'}_K, \mathbf{V'}_\text{s} \right]$. The idea of the proof is to construct $\mathbf{V}'$ so that it has the same covariance as $\mathbf{\hat{V}}$, i.e.,
        \begin{equation} \label{eq:cov_eq}
            \mathbf{V}' {\mathbf{V}'}^\mathsf{H} = \mathbf{\hat{V}} \mathbf{\hat{V}}^\mathsf{H},
        \end{equation}
        with the additional property that the communication beamformers of $\mathbf{V}'$ shall now contain all components in the directions of $\mathbf{h}_1, \ldots, \mathbf{h}_K$. To find such communication beamformers, we aim to maximize the minimum power in the directions of $\mathbf{h}_1, \ldots, \mathbf{h}_K$, weighted by a fixed interference level. Let $w_k \triangleq (1 + \tfrac{1}{\gamma_k}) \tfrac{1}{\mathbf{h}_k^\mathsf{H}\mathbf{\hat{V}}\mathbf{\hat{V}}^\mathsf{H} \mathbf{h}_k +  \sigma^2}$. We determine $\mathbf{v}_1', \ldots, \mathbf{v}_K'$ as a solution of
    \begin{subequations} \label{prob:max_min_pw}
\begin{align} \label{eq:max_min_obj} \underset{{\mathbf{v}_1, \ldots, \mathbf{v}_K}}{\mathrm{maximize}}  ~~&\min_k ~~ w_k |\mathbf{h}_k^\mathsf{H} \mathbf{v}_k|^2 \\
    \mathrm{subject \; to} ~~&\mathbf{\hat{V}}\mathbf{\hat{V}}^\mathsf{H} \succcurlyeq \sum_k \mathbf{v}_k \mathbf{v}_k^\mathsf{H}, \label{eq:max_min_const_a}
\end{align}
  \end{subequations}
        Once the communication beamformers are found, we obtain the sensing beamformers of $\mathbf{V}'$ using the difference between the overall covariance and the covariance of the communication beamformers, i.e.,
        \begin{equation}\label{eq:V_s_prime}
    \mathbf{V}_\text{s}' {\mathbf{V}_\text{s}'}^\mathsf{H} = \mathbf{\hat{V}}\mathbf{\hat{V}}^\mathsf{H} - \sum_k \mathbf{v}_k' {\mathbf{v}_k'}^\mathsf{H}.
        \end{equation}
       First, let us show that such $\mathbf{V}'$ is indeed an optimal solution of $\mathcal{P}_N^\text{NIC}$. The total power and BFIM are the same because they are both determined only by the overall covariance, which is fixed by~\eqref{eq:cov_eq}. The fact that the SINRs constraints are satisfied follows a two-step argument. First, we prove that the optimal value of  problem~\eqref{eq:max_min_obj} must be greater than or equal to one
    \begin{subequations}
        \begin{align}
            \min_k  w_k |\mathbf{h}_k^\mathsf{H} \mathbf{v}_k'|^2 & \geq \min_k w_k |\mathbf{h}_k^\mathsf{H} \mathbf{\hat{v}}_k|^2 \\
            &= \min_k  \left(1 + \frac{1}{\gamma_k} \right) \frac{|\mathbf{h}_k^\mathsf{H}\mathbf{\hat{v}}_k|^2}{\mathbf{h}_k^\mathsf{H}\mathbf{\hat{V}}\mathbf{\hat{V}}^\mathsf{H} \mathbf{h}_k +  \sigma^2} \\
            %&= \min_k  (1 + \frac{1}{\gamma_k}) \left( \frac{\mathbf{h}_k^\mathsf{H}\mathbf{\hat{V}}\mathbf{\hat{V}}^\mathsf{H} \mathbf{h}_k +  \sigma^2}{|\mathbf{h}_k^\mathsf{H}\mathbf{\hat{v}}_k|^2} \right)^{-1} \\
            &= \min_k  \left(1 + \frac{1}{\gamma_k} \right) \left(1 +  \frac{1}{\text{SINR}^\text{NIC}_{k, \mathbf{\hat{V}}}} \right)^{-1} \\
            & \geq \min_k ~ \left(1 + \frac{1}{\gamma_k}\right) \left(1 +  \frac{1}{\gamma_k} \right)^{-1} = 1
        \end{align}
        \end{subequations}
        where the last line follows since $\mathbf{\hat{V}}$ satisfies $\text{SINR}^\text{NIC}_{k, \mathbf{\hat{V}}} \geq \gamma_k$. Next, we prove that the SINR constraints must be satisfied for all $k$ since
    \begin{subequations}
        \begin{align}
            w_k |\mathbf{h}_k^\mathsf{H} \mathbf{v}_k'|^2 \geq 1 &\Leftrightarrow \left(1 + \frac{1}{\gamma_k}\right)  \geq \frac{\mathbf{h}_k^\mathsf{H}\mathbf{\hat{V}}\mathbf{\hat{V}}^\mathsf{H} \mathbf{h}_k +  \sigma^2}{|\mathbf{h}_k^\mathsf{H}\mathbf{v}'_k|^2} \\
            &\Leftrightarrow \left(1 + \frac{1}{\gamma_k} \right)  \geq \frac{\mathbf{h}_k^\mathsf{H}\mathbf{V}'{\mathbf{V}'}^\mathsf{H} \mathbf{h}_k +  \sigma^2}{|\mathbf{h}_k^\mathsf{H}\mathbf{v}'_k|^2} \label{eq:SINR_proof_line_b}\\& \Leftrightarrow \left(1 + \frac{1}{\gamma_k}\right)  \geq 1 + \frac{1}{\text{SINR}^\text{NIC}_{k, \mathbf{V}'}} \\
            & \Leftrightarrow \text{SINR}^\text{NIC}_{k, \mathbf{V}'} \geq \gamma_k.
        \end{align}
        \end{subequations}
        where in~\eqref{eq:SINR_proof_line_b}
        we used~\eqref{eq:cov_eq}. 
        Hence, $\mathbf{V}'$ satisfies the SINR constraints and is optimal for $\mathcal{P}_N^\text{NIC}$.

Note that $\mathbf{V}'$ obtained in the above manner is not unique. This is because the communication beamformers obtained by solving problem~\eqref{prob:max_min_pw} may not be unique. 
Next, we aim to show that there exists at least one $\mathbf{V}'$ whose sensing beamformers are orthogonal to $\mathbf{h}_1, \ldots, \mathbf{h}_K$. To do this, we first prove that problem~\eqref{prob:max_min_pw} has strong duality. This can be proved by showing that the SDR of problem~\eqref{prob:max_min_pw} is tight using the same trick from Appendix~\ref{Appen:strong_duality}. The convex SDR of problem~\eqref{prob:max_min_pw} is given by
\begin{subequations} \label{prob:max_min_pw_SDR}
\begin{align}
\underset{{\mathbf{R}_1 \succcurlyeq 0, \ldots, \mathbf{R}_K \succcurlyeq 0, t}}{\mathrm{maximize}}  ~~& t \\
    \mathrm{subject \; to} ~~~&\mathbf{\hat{V}}\mathbf{\hat{V}}^\mathsf{H} \succcurlyeq \sum_k \mathbf{R}_k, \label{eq:SDR_const_a} \\
    &  t \leq  w_k \Tr\left(\mathbf{R}_k \mathbf{h}_k \mathbf{h}_k^\mathsf{H}\right), \label{eq:SDR_const_b}
    %&\mathbf{R}_k \succcurlyeq 0, ~~ \forall k,
\end{align}
\end{subequations}
which is obtained by defining $\mathbf{R}_k = \mathbf{v}_k \mathbf{v}_k^\mathsf{H}$ and dropping the rank-one constraints. %The SDR is tight can be proved by proving the existence of a rank-one solution using the technique in~\cite{Liu2020joint}. 
Let $\mathbf{\hat{R}}_1, \ldots, \mathbf{\hat{R}}_K$ be an arbitrary high-rank solution of the SDR~\eqref{prob:max_min_pw_SDR}. Then, 
\begin{align}
    \mathbf{\tilde{R}}_k = \frac{\mathbf{\hat{R}}_k \mathbf{h}_k \mathbf{h}_k^\mathsf{H} \mathbf{\hat{R}}_k}{\mathbf{h}_k^\mathsf{H} \mathbf{\hat{R}}_k \mathbf{h}_k }, \quad \forall k.
\end{align}
are rank-one matrices satisfying
\begin{align}\label{eq:rank_one_conditions}
    \mathbf{\hat{R}}_k \succcurlyeq \mathbf{\tilde{R}}_k, \quad  \Tr\left(\mathbf{\hat{R}}_k \mathbf{h}_k \mathbf{h}_k^\mathsf{H}\right) = \Tr\left(\mathbf{\tilde{R}}_k \mathbf{h}_k \mathbf{h}_k^\mathsf{H}\right), \quad \forall k.
\end{align} 
The first condition in~\eqref{eq:rank_one_conditions} implies that $\sum_k \mathbf{\tilde{R}}_k \preccurlyeq \sum_k \mathbf{\hat{R}}_k \preccurlyeq \mathbf{\hat{V}}\mathbf{\hat{V}}^\mathsf{H}$, so that~\eqref{eq:SDR_const_a} is satisfied for the rank-one matrices $\mathbf{\tilde{R}}_1, \ldots, \mathbf{\tilde{R}}_K$.  The second condition implies that $\mathbf{\tilde{R}}_1, \ldots, \mathbf{\tilde{R}}_K$ attain the same optimal objective as $\mathbf{\hat{R}}_1, \ldots, \mathbf{\hat{R}}_K$.  Thus, $\mathbf{\tilde{R}}_1, \ldots, \mathbf{\tilde{R}}_K$ is a rank-one solution of~\eqref{prob:max_min_pw_SDR} and the SDR is tight. Strong duality follows by noting that problem~\eqref{prob:max_min_pw} and its SDR give rise to the same dual problem:
\begin{subequations}
    \begin{align}
    \underset{\mathbf{Z}, \mu_1, \ldots, \mu_K}{\mathrm{minimize}} ~~ &\Tr\left( \mathbf{Z} \mathbf{\hat{V}}\mathbf{\hat{V}}^\mathsf{H}  \right) \\
        \mathrm{subject \; to} ~~&\mathbf{Z} - \mu_k w_k \mathbf{h}_k \mathbf{h}_k^\mathsf{H} \succcurlyeq 0, ~~ \forall k. \label{eq:dual_const_b} \\
        &\mathbf{Z} \succcurlyeq 0, \quad \mu_k \geq 0, \quad \sum_k \mu_k = 1. \label{eq:dual_const_c}
    \end{align}
\end{subequations}
where $\mathbf{Z}$ and $\mu_k$ are the dual variables associated with~\eqref{eq:SDR_const_a} (or~\eqref{eq:max_min_const_a}) and~\eqref{eq:SDR_const_b}. Since the dual problem is convex with nonempty interior, we have strong duality for the SDR~\eqref{prob:max_min_pw_SDR}. Since the SDR is tight, problem~\eqref{prob:max_min_pw} also enjoys strong duality.

Such a strong duality result allows us to prove the existence of some $\mathbf{V}_\text{s}'$ orthogonal to $\mathbf{h}_1, \ldots, \mathbf{h}_K$ by analyzing a set of optimality conditions. Let  $\mathbf{v}_1', \ldots, \mathbf{v}_K'$ be a solution of problem~\eqref{prob:max_min_pw}. Then, there exist dual-optimal variables $\mathbf{Z}' \succcurlyeq 0$ and $\mu'_1, \ldots, \mu'_K$ such that the complementary condition
\begin{equation}\label{eq:CS_cond}
    \mathbf{Z}' \left(\mathbf{\hat{V}} \mathbf{\hat{V}}^\mathsf{H} - \sum_k \mathbf{v}_k' {\mathbf{v}_k'}^\mathsf{H} \right) = 0 \Leftrightarrow \mathbf{Z}' \mathbf{V}'_\text{s} {\mathbf{V}'_\text{s}}^\mathsf{H} = 0,
\end{equation}
holds. The right-hand-side condition in~\eqref{eq:CS_cond}  follows from~\eqref{eq:V_s_prime}. Combining~\eqref{eq:CS_cond} with the fact that $\mathbf{Z}'$ and $\mu_1', \ldots, \mu_K'$ must satisfy~\eqref{eq:dual_const_b}, we obtain for all $k$
\begin{subequations}
\begin{align}
    \mathbf{Z}' - \mu_k' w_k \mathbf{h}_k \mathbf{h}_k^\mathsf{H} \succcurlyeq 0, &~  \mathbf{Z}' \mathbf{V}'_\text{s} {\mathbf{V}'_\text{s}}^\mathsf{H} = 0 \\
    \Rightarrow & \mu_k' \Tr\left(\mathbf{h}_k \mathbf{h}_k^\mathsf{H} \mathbf{V}_\text{s}' {\mathbf{V}_\text{s}'}^\mathsf{H}\right) = 0. \label{eq:zero_condition}%~\forall k.
\end{align}
\end{subequations}
%In the rest of the proof, we ignore the remaining complementary conditions since~\eqref{eq:CS_cond} this is enough to prove the desired result. 
Suppose that $\mu_1', \ldots, \mu_K'$ are all strictly positive. Then, by~\eqref{eq:zero_condition}, we must have $\Tr(\mathbf{h}_k \mathbf{h}_k^\mathsf{H} \mathbf{V}_\text{s}' {\mathbf{V}_\text{s}'}^\mathsf{H}) = \|\mathbf{V}_\text{s}' \mathbf{h}_k \|_\text{F}^2 = 0$ for all $k$. %Since $\mathbf{V}_\text{s}'$ is not zero by assumption, 
This can only happen if $\mathbf{V}_\text{s}'$ is orthogonal to $\mathbf{h}_1, \ldots, \mathbf{h}_K$. 

Next, assume that there is a subset of $\left\{1, \ldots, K \right\}$ for which $\mu'_k = 0$. For convenience, we denote such set by $\mathcal{K} = \{k | \mu'_k = 0\}$ and its complement by $\mathcal{K}^\text{c} = \{k | \mu'_k > 0\}$. Note that $\mathcal{K}^\text{c}$ cannot be empty since $\mu_1', \ldots, \mu_K'$ sum up to one; see constraint~\eqref{eq:dual_const_c}. Therefore, there exists at least one $\mu'_k > 0$ with $|\mathcal{K}^\text{c}| \neq  0$ and $|\mathcal{K}| < K$. Due to complementary slackness, it can be verified that the $\{\mathbf{v}_k'\}$ with indices in $\mathcal{K}^\text{c}$ attain the minimum value in~\eqref{eq:max_min_obj}, whereas the $\{\mathbf{v}_k'\}$ with $k \in \mathcal{K}$ attain a potentially higher value than $\min_k w_k |\mathbf{h}_k^\mathsf{H} \mathbf{v}_k'|^2$. %This fact can be proved by examining the complementary conditions associated with $\mu_1', \ldots, \mu_K'$.

By~\eqref{eq:zero_condition}, it is easy to verify that \emph{any} $\mathbf{V}_\text{s}'$ is orthogonal to the $\{\mathbf{h}_k\}$ for the user indices in $\mathcal{K}^\text{c}$ (i.e., due to $\mu_k' > 0$). However, it is not necessarily true that such $\mathbf{V}_\text{s}'$ is orthogonal to the $\{\mathbf{h}_k\}$ for the user indices in $\mathcal{K}$. 
Nevertheless, we can prove the existence of \emph{at least one} such $\mathbf{V}_\text{s}'$ that is also orthogonal to all $\{\mathbf{h}_k\}$. The idea is to fix the communication beamformers that correspond to $k \in \mathcal{K}^\text{c}$ (i.e., the set for which $\mu_k' > 0$)  and define a new minimum power optimization similar to problem~\eqref{prob:max_min_pw} over the remaining beamformers. Let $\mathbf{\hat{W}} \mathbf{\hat{W}}^\mathsf{H} = \mathbf{\hat{V}} \mathbf{\hat{V}} - \sum_{k \in \mathcal{K}^\text{c}} \mathbf{v}_k' {\mathbf{v}_k'}^\mathsf{H}$ be the new covariance matrix and consider the following optimization.  
\begin{subequations}\label{prob:max_min_new}
\begin{align} \label{eq:max_min_obj_new} \underset{\{\mathbf{v}_i\}, i \in \mathcal{K} }{\mathrm{maximize}}  ~~&\min_{k \in \mathcal{K}} ~~ w_k |\mathbf{h}_k^\mathsf{H} \mathbf{v}_k|^2 \\
    \mathrm{subject \; to} ~~&\mathbf{\hat{W}}\mathbf{\hat{W}}^\mathsf{H} \succcurlyeq \sum_{k \in \mathcal{K}} \mathbf{v}_k \mathbf{v}_k^\mathsf{H}. 
\end{align}
  \end{subequations}
The new problem~\eqref{prob:max_min_new} is similar to problem~\eqref{prob:max_min_pw}, but over a strictly smaller set of communication beamformers given by $\{\mathbf{v}_k\}$ for $k \in \mathcal{K}$. %It can be verified that all previous statements that apply to problem~\eqref{prob:max_min_pw} are also applicable to the new optimization~\eqref{prob:max_min_new}. 
A solution of~\eqref{prob:max_min_new}, denoted by $\{\mathbf{v}_k''\}_{k \in \mathcal{K}}$,  together with the previously fixed beamformers $\{\mathbf{v}_k'\}_{k \in \mathcal{K}^\text{c}}$, 
constitutes a solution of the original problem~\eqref{prob:max_min_pw}. This is because the new beamformers $\{\mathbf{v}_k''\}_{k \in \mathcal{K}}$ will always attain power values that are higher than the minimum value attained by the fixed beamformers $\{\mathbf{v}_k'\}_{k \in \mathcal{K}^\text{c}}$ as perviously discussed.  In this case, we may choose $\mathbf{V}_\text{s}'$ as follows:
\begin{subequations}
\begin{align}
    \mathbf{V}_\text{s}' {\mathbf{V}_\text{s}'}^\mathbf{H} &= \mathbf{\hat{W}} \mathbf{\hat{W}}^\mathsf{H} - \sum_{k \in \mathcal{K}} \mathbf{v}_k'' {\mathbf{v}_k''}^\mathsf{H} \\
    &= \mathbf{\hat{V}} \mathbf{\hat{V}} - \sum_{k \in \mathcal{K}^\text{c}} \mathbf{v}_k' {\mathbf{v}_k'}^\mathsf{H} - \sum_{k \in \mathcal{K}} \mathbf{v}_k'' {\mathbf{v}_k''}^\mathsf{H}.
\end{align}
\end{subequations}
Such $\mathbf{V}_\text{s}'$ is orthogonal to $\{\mathbf{h}_k\}$ for $k \in \mathcal{K}^\text{c}$ by~\eqref{eq:zero_condition}. Now, the set of solutions to the new problem~\eqref{prob:max_min_new}
can be similarly divided into subsets corresponding to zero and nonzero optimal dual variables $\{\mu_k''\}$. Let $\mathcal{K}' = \{k \in \mathcal{K} | \mu''_k = 0\}$ and ${\mathcal{K}^\text{c}}' = \{k \in \mathcal{K} | \mu''_k > 0\}$. By similar arguments as before, the optimality conditions of the new problem~\eqref{prob:max_min_new} must also be satisfied for $\mu_k''$. This yields a similar condition to~\eqref{eq:zero_condition}, given by: %(see~\eqref{eq:zero_condition}).
\begin{subequations}
\begin{align}
    &\mu_k'' \Tr \left( \mathbf{h}_k \mathbf{h}_k^\mathsf{H}\left( \mathbf{\hat{W}}\mathbf{\hat{W}}^\mathsf{H} - \sum_{k \in \mathcal{K}} \mathbf{v}_k'' {\mathbf{v}_k''}^\mathsf{H} \right) \right) = 0 \\
    &\qquad \qquad \qquad \qquad  \Leftrightarrow  \mu_k'' \Tr\left( \mathbf{h}_k \mathbf{h}_k^\mathsf{H} \mathbf{V}_\text{s}' {\mathbf{V}_\text{s}'}^\mathsf{H} \right) = 0.
\end{align}
\end{subequations}
for all $k$. For the set of $k \in {\mathcal{K}^\text{c}}'$, we have $\mu_k'' > 0$. This implies that $ \mathbf{V}_\text{s}' \mathbf{h}_k = 0$ for $k \in {\mathcal{K}^\text{c}}' \cup \mathcal{K}^\text{c}$.
 
 Now, the new optimal dual variables $\{\mu_k''\}$ must also sum up to one. Therefore, the set ${\mathcal{K}^\text{c}}'$ cannot be empty, which implies that $|\mathcal{K}'| < |\mathcal{K}|$, i.e., the the set of user indices with channels that may not be orthogonal to the new $\mathbf{V}_\text{s}'$ is reduced. If $\mathcal{K}'$ is nonempty, the process can repeated iteratively. In each iteration, we define a new $\mathbf{\hat{W}}$ and solve the optimization~\eqref{prob:max_min_new} over a strictly smaller subset to obtain a new $\mathbf{V}_\text{s}'$. The process terminates when $\mathcal{K}'$ is empty. In this case, we have $\mathbf{V}_\text{s}' \mathbf{h}_k = 0, \forall k$.

\section{Proof of Lemma~\ref{lem:quad_eq_sol_NIC}}\label{appen:quad_eq_sol_NIC}
First, we prove the existence of $\mathbf{U}$ that conforms to~\eqref{eq:lin_transform_compact} and gives rise to some $\mathbf{V}'$ satisfying~\eqref{eq:BFIM_SINR_NIC}, if $N$ satisfies~\eqref{eq:main_cond_NIC}. To do this, we argue that the SINR constraints are automatically satisfied regardless of the choice of $\mathbf{U}$ in~\eqref{eq:lin_transform_compact}. 
To see why, we note that for any $i$ and $k$ in $\left\{1, \ldots, K \right\}$, we have
\begin{equation}
|\mathbf{h}_i^\mathbf{H} \mathbf{v}'_k|^2 = |\mathbf{h}_i^\mathbf{H} (\mathbf{\hat{v}}_k + \mathbf{\hat{V}}_\text{s}\mathbf{u}_k)|^2 = |\mathbf{h}_i^\mathbf{H} \mathbf{\hat{v}}_k|^2,
\end{equation}
which holds for all $\mathbf{u}_k$ since $\mathbf{\hat{V}}_\text{s}$ is chosen to be orthogonal to $\mathbf{h}_1, \ldots, \mathbf{h}_K$ as given by Lemma~\ref{lem:Ortho_Vs_NIC}. Likewise, it is easy to verify that $\mathbf{h}_k^\mathsf{H} \mathbf{V}_\text{s}'{\mathbf{V}'_\text{s}}^\mathsf{H} \mathbf{h}_K = \mathbf{h}_k^\mathsf{H} \mathbf{\hat{V}}_\text{s}\mathbf{\hat{V}}_\text{s}^\mathsf{H}  \mathbf{h}_K = 0$, for all $\mathbf{U}_\text{s}$. Therefore, any $\mathbf{U}_\text{c}$ and $\mathbf{U}_\text{s}$ (or $\mathbf{U}$ in~\eqref{eq:lin_transform_compact}), the SINR for the $k$-th user remains the same, i.e.,
\begin{subequations}
\begin{align}
\text{SINR}^\text{NIC}_{k, \mathbf{V}'} &= \frac{|\mathbf{h}_k^\mathsf{H} \mathbf{v}'_k|^2}{\sum_{i \neq k} |\mathbf{h}_k^\mathsf{H} \mathbf{v}'_i|^2 + \mathbf{h}_k^\mathsf{H} \mathbf{V}'_\text{s} {\mathbf{V}'_\text{s}}^\mathsf{H} \mathbf{h}_k + \sigma^2} \\
 &=  \frac{|\mathbf{h}_k^\mathsf{H} \mathbf{\hat{v}}_k|^2}{\sum_{i \neq k} |\mathbf{h}_k^\mathsf{H} \mathbf{\hat{v}}_i|^2 + \mathbf{h}_k^\mathsf{H} \mathbf{\hat{V}}_\text{s} {\mathbf{\hat{V}}_\text{s}}^\mathsf{H} \mathbf{h}_k + \sigma^2},  \\
 &=  \text{SINR}^\text{NIC}_{k, \mathbf{\hat{V}}} = \gamma_k',
\end{align}
\end{subequations}
for all $k$. %This shows that the SINRs are satisfied for all choices of $\mathbf{U}_\text{c}$ and $\mathbf{U}_\text{s}$.
Next, we focus on the BFIM. For the new $\mathbf{V}'$ to satisfy $\mathbf{J}_{\mathbf{V}'} = \mathbf{J} = \mathbf{J}_{\mathbf{\hat{V}}}$, we must have
\begin{align}
\Tr\left(\mathbf{\tilde{G}}_{ij} \mathbf{V}' {\mathbf{V}'}^\mathsf{H} \right) = \Tr\left(\mathbf{\tilde{G}}_{ij} \mathbf{\hat{V}} \mathbf{\hat{V}}^\mathsf{H} \right),
\end{align}
which is equivalent to
\begin{align}
\Tr\left(\mathbf{\tilde{G}}_{ij} \mathbf{\hat{V}} \left(\mathbf{I}_{N} - \mathbf{U} \mathbf{U}^\mathsf{H} \right) {\mathbf{\hat{V}}}^\mathsf{H} \right) = 0 \label{eq:quad_system_NIC} %\\
%& \qquad \qquad \qquad  \Leftrightarrow \Tr\left(\mathbf{\tilde{G}}_{ij} \mathbf{\hat{V}} \mathbf{M}{\mathbf{\hat{V}}}^\mathsf{H} \right) = 0, \label{eq:def_M}
\end{align}
for all $1 \leq i \leq j \leq L$. The system~\eqref{eq:quad_system_NIC} consists of $L (L + 1)/2$ quadratic equations in $\mathbf{U}$ that can be transformed into a linear system. Let $\mathbf{M} \triangleq \mathbf{I}_{N} - \mathbf{U} \mathbf{U}^\mathsf{H}$. We can  write~\eqref{eq:quad_system_NIC} as follows
\begin{equation}
\Tr\left(\mathbf{\tilde{G}}_{ij} \mathbf{\hat{V}} \mathbf{M}{\mathbf{\hat{V}}}^\mathsf{H} \right) = 0, \quad 1 \leq i \leq j \leq L. \label{eq:def_M}
\end{equation} %\\
%& \qquad \qquad \qquad  \Leftrightarrow \Tr\left(\mathbf{\tilde{G}}_{ij} \mathbf{\hat{V}} \mathbf{M}{\mathbf{\hat{V}}}^\mathsf{H} \right) = 0, \label{eq:def_M}
This is a linear system in $\mathbf{M}$. Additionally, $\mathbf{M}$ must satisfy the following %that arise based on how it is defined:
\begin{equation}\label{eq:extra_cond}
    \mathbf{I}_{N} -  \mathbf{M} \succcurlyeq 0, \quad \mathbf{I}_{N} - \mathbf{M}~ \text{singular}, ~~~ \mathbf{M} = \left[\begin{matrix} 
    \mathbf{0}_{K} & \mathbf{M}_{12}\\
\mathbf{M}_{12}^\mathsf{H} & \mathbf{M}_{22}\end{matrix} \right]
\end{equation}
for some arbitrary 
 $\mathbf{M}_{12}$ and $\mathbf{M}_{22}$. The first two conditions are self-explanatory and are similar to previous case in Lemma~\ref{lem:quad_eq_sol_IC}. The last condition is enforced since $\mathbf{U}$ has the form in~\eqref{eq:lin_transform_compact}. So that, $\mathbf{U} \mathbf{U}^\mathsf{H}$ has an identity matrix in the $K \times K$ top-left block, which translates to an all-zero matrix in the $K \times K$ top-left block of $M$.

Given $\mathbf{M}$ that satisfies~\eqref{eq:extra_cond}, it is always possible to recover $\mathbf{U}$ in the desired form. Indeed, since $\mathbf{I}_{N} - \mathbf{M}$ is PSD and singular, it must admit a compact decomposition $\mathbf{\tilde{U}} \mathbf{\tilde{U}}^\mathsf{H}$ for a tall matrix $\mathbf{\tilde{U}} \in \mathbb{C}^{\hat{N} \times N'}$. Since the $K \times K$ top-left block of $\mathbf{I}_{N} - \mathbf{M}$ is the identity matrix, the first $K$ rows of $\mathbf{\tilde{U}}$ must be orthonormal, i.e.,
\begin{equation}
    \mathbf{\tilde{U}} = \left[\begin{matrix}
        \mathbf{Q}_1 \\ \mathbf{Q}_2
    \end{matrix} \right], \quad \mathbf{Q}_1 \in \mathbb{C}^{K \times N'}, \quad \mathbf{Q}_1 \mathbf{Q}_1^\mathsf{H} = \mathbf{I}_K.
\end{equation}
It follows that there exist some $\mathbf{Q}_\perp \in \mathbb{C}^{(N' - K) \times N'}$ with $N' - K$ orthonormal rows such that $\mathbf{Q}_1 \mathbf{Q}_\perp^\mathsf{H} = \mathbf{0}$. We can then recover $\mathbf{U}$ as follows:
\begin{equation}
    \mathbf{U} = \mathbf{\tilde{U}} [\begin{matrix}
\mathbf{Q}_1^\mathsf{H} & \mathbf{Q}_\perp^\mathsf{H} \end{matrix}] = \left[ \begin{matrix}
    \mathbf{I}_K & \mathbf{0} \\
    \mathbf{Q}_2\mathbf{Q}_1^\mathsf{H} &  \mathbf{Q}_2\mathbf{Q}_\perp^\mathsf{H}
\end{matrix} \right]. 
\end{equation}
In particular, $\mathbf{U}_\text{c} = \mathbf{Q}_2\mathbf{Q}_1^\mathsf{H}$ and $\mathbf{U}_\text{s} = \mathbf{Q}_2\mathbf{Q}_\perp^\mathsf{H}$.

Now provided that~\eqref{eq:main_cond_NIC} holds, it is always possible to find $\mathbf{M}$ that satisfies both~\eqref{eq:def_M} and~\eqref{eq:extra_cond}. Indeed,~\eqref{eq:def_M} is a system of $L (L + 1)/2$ linear equations in $\mathbf{M}$, whereas $\mathbf{M}$ has $N^2 - K^2$ real unknowns since it is a $N \times N$ Hermitian matrix with a fixed $K \times K$ top-left block. Provided that~\eqref{eq:main_cond_NIC} holds, there are more real unknowns than equations and we can find a nonzero solution $\mathbf{M}'$. Such solution can then be scaled appropriately 
\begin{equation}
    \mathbf{M} = \frac{1}{\delta} \mathbf{M}', \quad |\delta| = \max\{|\delta_1'|, \ldots, |\delta_{\hat{m}}'|\}.
\end{equation}
to ensure that $\mathbf{I}_{N} - M$ is PSD and singular. %Here, $\delta_i$ is the $i$-th eigenvalue of $\mathbf{M}'$.

The proof of strong duality for $\mathcal{P}_{N'}^\text{NIC}$ is similar to that of Lemma~\ref{lem:quad_eq_sol_IC} and is omitted for brevity. %it can be shown that $\mathbf{V}'$ also attains the same power as $\mathbf{\hat{V}}$ since the latter is the minimum power solution of $\mathcal{P}_{\hat{N}}^\text{NIC}$, which has strong duality using the technique in~\cite{Liu2020joint}. This also implies that $\mathbf{V}'$ attains the minimum power of $\mathcal{P}_{N'}^\text{NIC}$ and that the latter problem itself enjoys strong duality. We omit the details for brevity. 
Note that $\mathbf{V}_\text{s}'$ is orthogonal to $\mathbf{h}_1, \ldots, \mathbf{h}_K$ since it is given by a linear map of $\mathbf{\hat{V}}_\text{s}$. 
\section{Two Beamformers Needed for Single Target Parameter Estimation}\label{appen:counter_example}
Consider the one target scenario with no users
\begin{equation}
    \mathbf{G}^{(\boldsymbol{\eta})} = \alpha \mathbf{a}_\text{R}(\theta)\mathbf{a}_\text{T}^\mathsf{H}(\theta).
\end{equation}
We show that one beamformer is not always sufficient to achieve the best possible estimation performance. Assume that the steering vectors are that of a uniform linear array
whose center is taken as a reference point~\cite{bekkerTarget2006, Li2008range}. Then, $\mathbf{a}_\text{T}(\cdot)$ and its derivative are given by
\begin{align}
    \mathbf{a}_\text{T}(\theta) &= \frac{1}{\sqrt{N_\text{T}}}\left[e^{-\imath \frac{N_\text{T} - 1}{2} \pi \sin(\theta)}, \ldots,   e^{\imath \frac{N_\text{T} - 1}{2} \pi \sin(\theta)} \right]^\mathsf{T} \\
    \mathbf{\dot{a}}_\text{T}(\theta) &= \frac{\imath \pi \cos{\theta} }{\sqrt{N_\text{T}}}\left[- \frac{N_\text{T} - 1}{2} a_1, \ldots, \frac{N_\text{T} - 1}{2} a_{N_\text{T}} \right],
 %e^{-\imath \frac{N_\text{D} - 1}{2} \pi \sin(\theta)}, \ldots,   e^{\imath \frac{N_\text{D} - 1}{2} \pi \sin(\theta)} \right]^\mathsf{T}, 
\end{align}
where $a_i$ is the $i$-th element of $\mathbf{a}_\text{D}(\theta)$ we adopt similar expressions for $\mathbf{a}_\text{R}(\cdot)$. Note that $\mathbf{\dot{a}}_\text{T}(\theta)$ and $\mathbf{a}_\text{T}(\theta)$ are orthogonal, i.e., $\mathbf{\dot{a}}_\text{T}^\mathsf{H}(\theta) \mathbf{a}_\text{T}(\theta) = 0$. Furthermore, it can be verified that
$\| \mathbf{a}_\text{T}(\theta) \|^2 = 1$, 
  and $\| \mathbf{\dot{a}}_\text{T}(\theta) \|^2 = \tfrac{\pi^2 \cos^2{\theta}}{12} (N_\text{T}^2 - 1)$. 

Let us consider the classical CRB as a special case for $\alpha = 1$ and arbitrary $\theta$. The trace of the CRB matrix is
\begin{align}
\Tr\left( \mathbf{J}_\mathbf{V}^{-1} \right) &= \frac{\Tr( \mathbf{\tilde{G}}_1 \mathbf{V} \mathbf{V}^\mathsf{H} ) + \Tr( \mathbf{\tilde{G}}_2 \mathbf{V} \mathbf{V}^\mathsf{H} )}{\Tr( \mathbf{\tilde{G}}_1 \mathbf{V} \mathbf{V}^\mathsf{H} ) \Tr( \mathbf{\tilde{G}}_2 \mathbf{V} \mathbf{V}^\mathsf{H} ) - |\Tr(\mathbf{\tilde{G}}_3 \mathbf{V}\mathbf{V}^\mathsf{H}) |^2 }  \nonumber \\
&~~~~+ \frac{1}{\Tr( \mathbf{\tilde{G}}_1 \mathbf{V} \mathbf{V}^\mathsf{H} )}
\end{align}
where $\mathbf{\tilde{G}}_1 = \mathbf{a}_\text{T} \mathbf{a}_\text{T}^\mathsf{H}$, $\mathbf{\tilde{G}}_2 = \| \mathbf{\dot{a}}_\text{R} \|^2 \mathbf{a}_\text{T} \mathbf{a}_\text{T}^\mathsf{H} + \mathbf{\dot{a}}_\text{T} \mathbf{\dot{a}}_\text{T}^\mathsf{H}$, and  $\mathbf{\tilde{G}}_3 = \mathbf{\dot{a}}_\text{T} \mathbf{a}_\text{T}^\mathsf{H}$. We drop the dependence on $\theta$ to simplify the notation. %Note that $\{\mathbf{\tilde{G}}_i\}$ depend only on $\mathbf{a}_\text{T}$ and $\mathbf{\dot{a}}_\text{T}$.

We aim to show that one beamformer is not always sufficient for certain values of $N_\text{T} > N_\text{R}$. To this end, our goal is to prove that the optimal value of the problem improves
\begin{equation} \label{prob:dummy_prob}
    \underset{\mathbf{V} \in \mathbb{C}^{N_\text{T} \times N}}{\mathrm{minimize}}~~ \Tr(\mathbf{J}_\mathbf{V}^{-1}) \quad \mathrm{s. \; t.}~ \Tr\left(\mathbf{V} \mathbf{V}^\mathsf{H} \right) \leq P.
\end{equation}
 if $N = 2$ beamformers are used, provided that $N_\text{T}, N_\text{R}$ satisfy
\begin{equation}\label{eq:cond_rank_2}
    N_\text{T}^2 > N_\text{R}^2 +  \frac{2\pi^2 \cos^2(\theta)}{12} (N_\text{R}^2 - 1)^2.
\end{equation}
To show this, first note that the value of the objective~\eqref{prob:dummy_prob} for some beamformer $\mathbf{v}_{\boldsymbol{\beta}} = \sqrt{\beta_1} \mathbf{a}_\text{T} + 
\sqrt{\beta_2} \mathbf{\dot{a}}_\text{T}$ is no better than that of the two beamformers $\mathbf{V}_{\boldsymbol{\beta}} = \left[ \begin{matrix} \sqrt{\beta_1} \mathbf{a}_\text{T} & \sqrt{\beta_2} \mathbf{\dot{a}}_\text{T} \end{matrix} \right]$, because %, by the fact that $\mathbf{a}_\text{T}$ and $\mathbf{a}_\text{R}$ are orthogonal, 
%$\mathbf{v}_{\boldsymbol{\beta}}$ and $\mathbf{V}_{\boldsymbol{\beta}}$ attain the same
$\Tr(\mathbf{\tilde{G}}_1 \mathbf{v}_{\boldsymbol{\beta}} \mathbf{v}_{\boldsymbol{\beta}}^\mathsf{H}) = \Tr(\mathbf{\tilde{G}}_1 \mathbf{V}_{\boldsymbol{\beta}} \mathbf{V}_{\boldsymbol{\beta}}^\mathsf{H}) = \beta_1$ and $\Tr(\mathbf{\tilde{G}}_2 \mathbf{v}_{\boldsymbol{\beta}} \mathbf{v}_{\boldsymbol{\beta}}^\mathsf{H})  = \Tr(\mathbf{\tilde{G}}_2 \mathbf{V}_{\boldsymbol{\beta}} \mathbf{V}_{\boldsymbol{\beta}}^\mathsf{H}) = \beta_1  \| \mathbf{\dot{a}}_\text{R} \|^2 + \beta_2  \| \mathbf{\dot{a}}_\text{T} \|^4$, but %$\mathbf{v}_{\boldsymbol{\beta}}$ achieving a larger value of
\begin{equation}\label{eq:G3_quad}
    \Tr(\mathbf{\tilde{G}}_3 \mathbf{v}_{\boldsymbol{\beta}} \mathbf{v}_{\boldsymbol{\beta}}^\mathsf{H}) = \sqrt{\beta_1 \beta_2} \| \mathbf{\dot{a}}_\text{T} \|^2  \geq 0 = \Tr(\mathbf{\tilde{G}}_3 \mathbf{V}_{\boldsymbol{\beta}} \mathbf{V}_{\boldsymbol{\beta}}^\mathsf{H}).
\end{equation}
Further, the objective strictly improves whenever $\beta_1 \beta_2 > 0$. 

Now, let ${\mathbf{v}^*}$ and $\mathbf{V}^*$ be the optimal solutions of~\eqref{prob:dummy_prob} when $N = 1$ and $N = 2$, respectively.  Suppose~\eqref{eq:cond_rank_2} holds.  Then,
\begin{align}
    \Tr(\mathbf{J}_{\mathbf{v}*}^{-1}) &= \min_{\beta_1, \beta_2 }  \Tr(\mathbf{J}_{\mathbf{v}_{\boldsymbol{\beta}} }^{-1}) \quad  \mathrm{s.t.} ~~ \beta_1 + \beta_2 \| \mathbf{\dot{a}}_\text{T} \|^2 \leq P \label{eq:equality_min} \\
  &> \min_{\beta_1, \beta_2 }  \Tr(\mathbf{J}_{\mathbf{V}_{\boldsymbol{\beta}} }^{-1}) \quad  \mathrm{s.t.} ~~ \beta_1 + \beta_2 \| \mathbf{\dot{a}}_\text{T} \|^2 \leq P  \label{eq:inequality_min} \\
  &= \Tr\left(\mathbf{J}_{\mathbf{V}^*}^{-1}\right) \label{eq:equality_min_2}
\end{align}
where equality in~\eqref{eq:equality_min} and~\eqref{eq:equality_min_2} follows by restricting the optimization to the subspace spanned by $\{\mathbf{a}_\text{T}, \mathbf{\dot{a}}_\text{T}\}$, since any other direction does not impact the CRB. We have strict equality in the second line since problem~\eqref{eq:inequality_min} has a solution satisfying $\beta_1^* \beta_2^* > 0$. Indeed, such problem is equivalent to 
\begin{equation}
    \min_{\beta_1, \beta_2}  ~ \frac{2}{\beta_1} + \frac{1}{\beta_1  \| \mathbf{\dot{a}}_\text{R} \|^2 + \beta_2  \| \mathbf{\dot{a}}_\text{T} \|^4} \quad  \mathrm{s.t.} ~~ \beta_1 + \beta_2 \| \mathbf{\dot{a}}_\text{T} \|^2 \leq P, 
\end{equation}
which is a convex problem. The optimal $\beta_1^*$ and $\beta_2^*$ are
\begin{equation}
    \beta_1^* = \min\left\{\frac{P \| \mathbf{\dot{a}}_\text{T} \|^2}{c +\sqrt{c/2}}, P\right\}, \quad \beta_2^* = \frac{1}{\| \mathbf{\dot{a}}_\text{T} \|^2} (P - \beta_1^*),
\end{equation}
where $c = \| \mathbf{\dot{a}}_\text{T} \|^2 - \| \mathbf{\dot{a}}_\text{R} \|^2 = \frac{\pi^2 \cos^2(\theta)}{12}  (N_\text{T}^2 - N_\text{R}^2)$. On the other hand, condition~\eqref{eq:cond_rank_2} ensures that  
\begin{align}
   c > \frac{2\pi^4 \cos^4(\theta)}{12^2} (N_\text{R}^2 - 1)^2  &\Leftrightarrow  \sqrt{c/2} > \frac{\pi^2 \cos^2(\theta)}{12} (N_\text{R}^2 - 1) \nonumber \\
   & \Leftrightarrow c + \sqrt{c/2} > \| \mathbf{\dot{a}}_\text{T} \|^2.
\end{align}
So that both $\beta_1^*$ and $\beta^*_2$ are strictly positive. This shows the existence of problem instances where a single beamformer is not enough to attain the best possible estimation performance for the one-target case.
